# Supplementary material for: DN-DETR: Accelerate DETR Training by Introducing Query DeNoising
Source: arXiv:2203.01305 source file (2022-12-08)
Supplement: Supplementary file 1 [file supp.tex]

\begin{table*}[ht]
    \centering
    %     \footnotesize
    %         \renewcommand{\arraystretch}{1.6}
    % \resizebox{\columnwidth}{!}{%
    \resizebox{1\textwidth}{!}{%
    \begin{tabular}{lccccccccccc}
        \toprule
        Model & MultiScale & \#epochs & AP & AP$_{50}$ & AP$_{75}$ & AP$_{S}$ & AP$_{M}$ & AP$_{L}$ & GFLOPs & Params \\
        \midrule
        DAB-DETR-DC$5$-R$50$    & & $50$ & {${44.5}$} & $65.1$ & $47.7$ & $25.3$ & $48.2$ & $62.3$ & $202$ & $44$M \\
        DN-DETR-DC$5$-R$50$    & &25 &$44.4$& $65.5$ & $50.8$ & $28.9$ & $50.2$ & $62.5$ & $202$ & $44$M\\
        \hline
        DAB-Deformable-DETR-R$50$    &\checkmark & $50$ & {$46.9$} & $66.0$ & $50.8$ & $30.1$ & $50.4$ & $62.5$ & $195$ & $48$M \\
        DN-Deformable-DETR-R$50$    & \checkmark&25 &$46.8$& $65.5$ & $50.8$ & $28.9$ & $50.2$ & $62.5$ & $195$ & $48$M\\
        \bottomrule
    \end{tabular}}
    
    \centering
    \caption{Results of our method trained for $25$ epochs and our baseline method trained for $50$ epochs under the same settings. The results shows we achieve $2$x acceleration with denoising training.
    }
    % \vspace{-0.4cm}
    \label{tab:speedup}
    % \vspace{-.3cm}
\end{table*}
